# Supplementary material for: Metallic Spin Liquid-like Behavior of LiV$_2$O$_4$
Source: arXiv:1812.05843 source file (2018-12-14)
Supplement: Supplementary file 1 [file lvo-msl-suppl-v2.pdf]

# Supplemental Material

H. Okabe,[1,2,3] M. Hiraishi,[1,2] A. Koda,[1,2,3] K. M. Kojima,[1,2,3] S. Takeshita,[1,2]
I. Yamauchi,[4] Y. Matsushita,[5] Y. Kuramoto,[2,6] and R. Kadono[1,2,3]

[1]*Muon Science Laboratory, Institute of Materials Structure Science, High Energy Accelerator Research Organization (KEK), Tsukuba, Ibaraki 305-0801, Japan*
[2]*Condensed Matter Research Center, Institute of Materials Structure Science, High Energy Accelerator Research Organization (KEK), Tsukuba, Ibaraki 305-0801, Japan*
[3]*The Graduate University for Advanced Studies (Sokendai), Tsukuba, Ibaraki 305-0801, Japan*
[4]*Department of Physics, Graduate School of Science and Engineering, Saga University, Saga 840-8502, Japan*
[5]*National Institute for Materials Science (NIMS), Tsukuba, Ibaraki 305-0044, Japan*
[6]*Department of Physics, Kobe University, Kobe 657-8501, Japan*

## I. SAMPLES

$LiV_2O_4$ samples for the present $\mu$SR experiment were synthesized by conventional solid state reaction under a reducing atmosphere. Since the sample was sensitive to air, the starting mixture and the heated products were handled in a glove box filled with dry argon gas. Pellets of stoichiometric mixture of $Li_3VO_4$, $V_2O_3$, and $V_2O_5$, were put into an evacuated quartz tube, and the tube was heated at 800 °C for 48 hours. The starting materials; $Li_3VO_4$ and $V_2O_3$ were synthesized the following manner. $Li_3VO_4$ was prepared from stoichiometric mixture of $Li_2CO_3$ (4N, Kojundo Chem. Co., Ltd.) and $V_2O_5$ (4N, Kojundo Chem. Co., Ltd.) under air at 800 °C for 72 hours, $V_2O_3$ was applied to the reduced process from $V_2O_5$ with flowing pure $H_2$ gas at 900 °C for a night. The obtained compound was an aggregate of randomly oriented micro-crystals ($10^0$–$10^1$ $\mu$m in size) with black color, which was pressed into a pellet for the ease of loading to cryostat.

Sample quality was examined using a part of these microcrystals. The phase purity was investigated by powder x-ray diffraction, where the data were obtained using a diffractometer with Cu $K_{\alpha 1}$ radiation (Rigaku SmartLab). The sample was confirmed to be highly monophasic. Magnetic data were collected using a SQUID magnetometer (MPMS-XL, Quantum Design Co. Ltd.). As shown in Fig. S1, magnetic susceptibility does not exhibit Curie-Weiss-like upturn at low temperatures, indicating that the present sample is free from magnetic impurities and defects in the crystal structure [1].

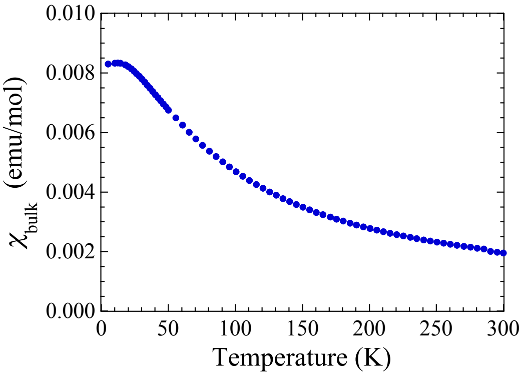


FIG. S1. Magnetic susceptibility of the $LiV_2O_4$ sample used for the present $\mu$SR experiment.

Meanwhile, the samples used for the previous specific heat measurement (the data quoted in Fig. 2d of the main text) were grown by a flux method with the eutectic solvent in LiCl–$Li_2MoO_4$–$LiBO_2$. The grown crystals show shiny black octahedral form having well developed [111] faces, and its sizes of up to 1 mm across corners. Chemical analysis using ICP revealed stoichiometric compositions. Details of the crystal growth, chemical and physical properties, and crystal structure are reported elsewhere [2, 3].

## II. $\mu$SR EXPERIMENT

Conventional $\mu$SR experiment was conducted using the GPS spectrometer at the Paul Scherrer Institute (PSI), where a muon beam with spin-polarization oriented 45° off the beam direction ($\hat{z}$) was implanted to the randomly oriented microcrystals of $LiV_2O_4$ samples (see the previous section for more detail). The two sets of time-dependent positron decay asymmetry $\mathcal{A}_\alpha(t)$ along the axes parallel ($\alpha = z$; longitudinal field, LF) and perpendicular ($\alpha = x$; transverse field, TF) to an external field $B_0$ ($\parallel \hat{z}$) were measured simultaneously by the corresponding positron detectors. These time spectra were analyzed by the least-square curve-fit in time domain using the respective recursive functions,

$$\mathcal{A}_z(t) = \mathcal{A}_{z0} \exp(-t/T_1^\mu)$$

for the LF, and

$$\mathcal{A}_x(t) = \sum_i \mathcal{A}_i \cos(\omega_{\mu i} t + \phi) \exp(-t/T_2^{\mu i})$$

for the TF spectra, where $\omega_{\mu i}$ and $1/T_2^{\mu i}$ are the muon spin precession frequency and transverse depolarization rate for the $i$-th component, $\phi$ is the initial phase of precession, and $\mathcal{A}_i$ is the partial asymmetry. The Knight shift for the TF spectra is defined by $K_{\mu i} \equiv (\omega_{\mu i} - \gamma_\mu B_0)/\gamma_\mu B_0$ with $\gamma_\mu = 2\pi \times 135.53$ MHz/T being the muon gyromagnetic ratio.

## III. HYPERFINE PARAMETERS

The hyperfine interaction between muon and electron is dominated by magnetic dipolar interaction in comparison to the Fermi contact interaction, because the latter, which is proportional to the probability of finding electron at the muon position $|\psi(0)|^2$, is small due to the small electric charge of muon ($e^+$) located at the interstitial site. In this situation, the hyperfine parameter is predominantly determined by the magnetic dipolar field $\boldsymbol{B}_{\rm dip}$ exerted by electrons (paramagnetic ions) which is calculated using the dipolar tensor $\mathbf{A}_i^{\rm dip}$,

$$\boldsymbol{B}_{\rm dip} = \sum_i \mathbf{A}_i^{\rm dip}\boldsymbol{\mu}_i = \sum_i\sum_\beta(\mathbf{A}_i^{\rm dip})_{\alpha\beta}(\boldsymbol{\mu}_i)^\beta, \quad (1)$$

$$(\mathbf{A}_i^{\rm dip})_{\alpha\beta} = \frac{1}{r_i^3}\left(\frac{3\alpha_i\beta_i}{r_i^2} - \delta_{\alpha\beta}\right), \quad (2)$$

where $\boldsymbol{r}_i = (x_i, y_i, z_i)$ is the position vector from muon to the $i$-th paramagnetic ion with the magnetic moment $\boldsymbol{\mu}_i$, and $\alpha,\beta = x,y,z$ [with $(\boldsymbol{\mu}_i)^\beta$ being its $\beta$ component] [4]. Thus the muon hyperfine parameter is given by $\mathbf{A}^{\rm dip} = \sum_i(\mathbf{A}_i^{\rm dip})$ when $|\boldsymbol{\mu}_i|$ is expressed in the unit of the Bohr magneton ($\mu_{\rm B}$). The $\mathbf{q}$-dependent hyperfine parameters ($A_{\mu\mathbf{q}}$) are obtained by the Fourier transform of Eq. (2).

The hyperfine parameter for longitudinal depolarization is given by the sum of the second moment for the transverse components of Eq. (2),

$$(\delta_\mu^{\parallel})^2 = \gamma_\mu^2\sum_i\sum_{\alpha,\beta}[(\mathbf{A}_i^{\rm dip})_{\alpha\beta}]^2, \quad (3)$$

where the sum runs except for the $zz$ component. The dipole tensor for muon occupying 16$c$ site in $\mathrm{LiV_2O_4}$ is calculated to be

$$\mathbf{A}^{\rm dip} = \begin{pmatrix} 0 & -95.74 & -95.74 \\ -95.74 & 0 & -95.74 \\ -95.74 & -95.74 & 0 \end{pmatrix} [\mathrm{mT}/\mu_{\rm B}], \quad (4)$$

which yields

$$\delta_\mu^{\parallel} = \gamma_\mu \times 0.2345\ \mathrm{T}/\mu_B = 199.7\ \mathrm{MHz}/\mu_B. \quad (5)$$

In the case of randomly oriented samples, further approximative treatment may be allowed to presume that

$$(\delta_\mu^{\parallel})^2 \simeq \gamma_\mu^2[\langle A_{xx}^2\rangle + \langle A_{yy}^2\rangle] = 2(\delta_\mu)^2, \quad (6)$$

$$(\delta_\mu^{\perp})^2 \simeq \gamma_\mu^2\langle A_{zz}^2\rangle^2 = (\delta_\mu)^2, \quad (7)$$

where $\delta_\mu$ is defined by

$$\gamma_\mu^2\langle A_{xx}^2\rangle = \gamma_\mu^2\langle A_{yy}^2\rangle = \gamma_\mu^2\langle A_{zz}^2\rangle \equiv (\delta_\mu)^2. \quad (8)$$

We use the above definition of $\delta_\mu$ for the hyperfine parameter in the main text, where $1/T_1^\mu$ is given by $2(\delta_\mu^{\rm L})^2$ with $\delta_\mu^{\rm L} = \delta_\mu = \delta_\mu^{\parallel}/\sqrt{2} = 141.2\ \mathrm{MHz}/\mu_B$.

The frequency spectra for the transverse spin precession in randomly oriented samples is generally described by the powder pattern, in which the Knight shift is determined by the principal value of diagonalized $\mathbf{A}^{\rm dip}$ [5]. Considering the axial symmetry of the 16$c$ site in $\mathrm{LiV_2O_4}$, the principal value corresponds to $A_\perp = +95.74\ \mathrm{mT}/\mu_B$, with which we have $K_\mu = A_\perp\chi/N_A\mu_B$. While this evaluation is qualitatively consistent with experimental observation (in the sign and orders of magnitude), the fact that $K_\mu$ is not proportional to the uniform susceptibility ($\chi_{\rm bulk}$) and that the linewidth exhibits significant field-induced broadening suggest that $K_\mu$ is not simply determined by the powder average. Therefore, we adopt the evaluation based on Eqs. (6)–(8), and assume that the shift is related with $\delta_\mu^\perp$. Then, we have $(\delta_\mu^\perp)^2 = (\delta_\mu^{\rm L})^2$, and $\gamma_\mu A_{\mu 0} \simeq \delta_\mu^\perp \simeq 141.2\ \mathrm{MHz}/\mu_B$ (or $A_{\mu 0} \simeq \delta_\mu^\perp/\gamma_\mu \simeq 165.8\ \mathrm{mT}/\mu_B$).

## IV. DYNAMICAL SPIN SUSCEPTIBILITY

We adopted single pole approximation for the dynamical spin susceptibility,

$$\chi(\mathbf{q},\omega) = \frac{\chi_{\rm s}}{1 + \dfrac{(\mathbf{q}-\mathbf{Q}_c)^2}{\kappa^2} - i\dfrac{\omega}{\Gamma(\mathbf{q})}}, \quad (9)$$

where $\chi_{\rm s} = \chi(\mathbf{Q}_c, 0)$ denotes the static susceptibility, $\mathbf{Q}_c$ is the $\mathbf{q}$-vector characterizing the antiferromagnetic spin fluctuation, $\kappa$ is the inverse correlation length of the fluctuation, and $\Gamma(\mathbf{q})$ is the $\mathbf{q}$-dependent spin fluctuation rate. Considering that the Knight shift and longitudinal spin depolarization rate are respectively related to the real and imaginary parts of $\chi(\mathbf{q},\omega)$, it is convenient to express $\chi(\mathbf{q},\omega)$ as follows:

$$\chi(\mathbf{q},\omega) = \chi'(\mathbf{q},\omega) + i\chi''(\mathbf{q},\omega), \quad (10)$$

where the respective components have the following explicit forms,

$$\chi'(\mathbf{q},\omega) = \frac{\chi_{\rm s}\left[1 + \frac{(\mathbf{q}-\mathbf{Q}_c)^2}{\kappa^2}\right][\Gamma(\mathbf{q})]^2}{\omega^2 + \left[1 + \frac{(\mathbf{q}-\mathbf{Q}_c)^2}{\kappa^2}\right]^2[\Gamma(\mathbf{q})]^2}, \quad (11)$$

$$\chi''(\mathbf{q},\omega) = \frac{\chi_{\rm s}\omega\Gamma(\mathbf{q})}{\omega^2 + \left[1 + \frac{(\mathbf{q}-\mathbf{Q}_c)^2}{\kappa^2}\right]^2[\Gamma(\mathbf{q})]^2}. \quad (12)$$

In the simplest case of single $\chi(\mathbf{q},\omega)$ component, the Knight shift ($K_a$) and longitudinal spin depolarization rate ($1/T_1^a$) in the low frequency limit (i.e., $\omega_a \ll \Gamma$) are related to $\chi(\mathbf{q},\omega)$ as

$$K_a = \frac{A_{a0}}{N_A\mu_B}\chi'(0,0) \simeq \frac{A_{a0}}{N_A\mu_B}\frac{\chi_{\rm s}}{1+|\mathbf{Q}_c|^2/\kappa^2}, \quad (13)$$

$$1/T_1^a = \frac{k_BT}{N_A\mu_B^2}\sum_{\mathbf{q}}(\gamma_a A_{a\mathbf{q}})^2\frac{\chi''(\mathbf{q},\omega_a)}{\omega_a} \quad (14)$$

$$\simeq \frac{k_BT}{N_A\mu_B^2}\chi_{\rm s}\sum_{\mathbf{q}}\frac{(\gamma_a A_{\mu\mathbf{q}})^2\Gamma(\mathbf{q})}{\omega_a^2 + \left[1 + \frac{(\mathbf{q}-\mathbf{Q}_c)^2}{\kappa^2}\right]^2[\Gamma(\mathbf{q})]^2},$$

where $A_{a\mathbf{q}}$ is the $\mathbf{q}$-dependent hyperfine parameters.

In the case of $LiV_2O_4$, the model is expanded to allow two components for $\chi(\mathbf{q}, \omega)$ (discerned by $\sigma$ = F, L),

$$\chi(\mathbf{q}, \omega) = \sum_{\sigma=\mathrm{F,L}} \chi_\sigma(\mathbf{q}, \omega) = \sum_{\sigma=\mathrm{F,L}} [\chi'_\sigma(\mathbf{q}, \omega) + i\chi''_\sigma(\mathbf{q}, \omega)], \quad (15)$$

and we have

$$K_a = \frac{1}{N_A \mu_B} \sum_{\sigma=\mathrm{F,L}} A^\sigma_{a0}\chi_\sigma(0,0) \simeq \frac{1}{N_A \mu_B} \sum_{\sigma=\mathrm{F,L}} \frac{A^\sigma_{a0}\chi_{\sigma s}}{1 + |\mathbf{Q}_c|^2/(\kappa^\sigma)^2} \quad (16)$$

$$1/T^a_1 = \frac{k_B T}{N_A \mu_B^2} \sum_{\mathbf{q},\sigma=\mathrm{F,L}} \frac{(\gamma_a A^\sigma_{a\mathbf{q}})^2 \chi_{\sigma s} \Gamma^\sigma(\mathbf{q})}{\omega_a^2 + \left[1 + \frac{(\mathbf{q}-\mathbf{Q}_c)^2}{(\kappa^\sigma)^2}\right]^2 [\Gamma^\sigma(\mathbf{q})]^2}, \quad (17)$$

where $A^\sigma_{a\mathbf{q}}$ is the $\mathbf{q}$- and $\sigma$-dependent hyperfine parameters. Because of the mutually complementary coupling of $A^\sigma_{a\mathbf{q}}$ to $\chi_\sigma(\mathbf{q}, \omega)$ between $\mu$SR ($a = \mu$) and $^7$Li-NMR ($a = I$), the F (L) component for Eqs. (16) and (17) is presumed to have negligible contributions to $K_\mu$, $1/T^\mu_1$ ($K_I$, $1/T^I_1$).

## V. SENSITIVE RANGE OF $1/T_1$ VS SPIN FLUCTUATION RATE

As shown in the main text, the longitudinal depolarization rate is approximated by $\mathbf{q}$-averaging to yield

$$\frac{1}{T^a_1 T} \simeq \frac{k_B}{N_A \mu_B^2} \sum_{\sigma=\mathrm{F,L}} \frac{2(\delta^\sigma_a)^2 \chi^\sigma_s \nu^\sigma}{\omega_a^2 + (\nu^\sigma)^2} \quad (18)$$

where $2(\delta^\sigma_a)^2$ and $\nu^\sigma$ are the $\mathbf{q}$-averaged quantities for $(\gamma_a A^\sigma_{a\mathbf{q}})^2$ and $\Gamma^\sigma(\mathbf{q})$.

While $\mu$SR and NMR can be used to observe the spin fluctuation via the same process described by Eq. (18), their sensitive ranges are markedly different. As illustrated in Fig. S2, the difference stems from that in the accessible time window, $T_\mathrm{W}$, for the respective probes (see also Table I). According to the earlier literatures on $^7$Li-NMR, the reported $1/T_1$ for $LiV_2O_4$ seems to exhibit an upper boundary of $\sim 10^2$ s$^{-1}$, above which $\mu$SR becomes a feasible technique to measure $1/T_1$. The present study benefits greatly from this unique sensitive range of $\mu$SR to spin fluctuation.

Another important factor is that Eq. (18) is a double-valued function in terms of $\nu$, where the peak of $1/T_1$ is given by the condition $\omega_a = \nu$. The situation of fast fluctuation ($\nu \gg \omega_a$) is conventionally called "motional narrowing" where $1/T_1$ is inversely proportional to $\nu$, while the opposite limit is called "motional broadening." Whether or not the fluctuation is in the "motional narrowing" limit is readily judged by the field ($\omega_a$) dependence of $1/T_1$, as $1/T_1$ is independent of $\omega_a$ ($\ll \nu$) in the motional narrowing limit whereas it is strongly dependent on $\omega_a$ in the opposite case.

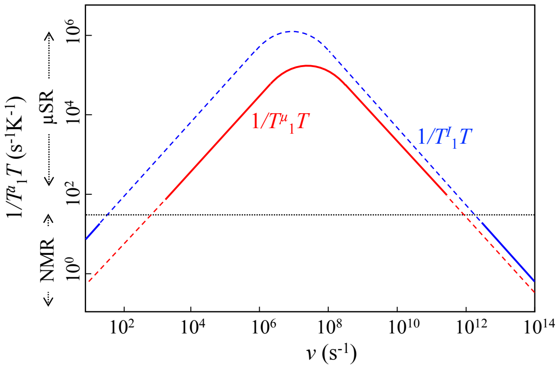


FIG. S2. Schematic illustration of $1/T^a_1T$ versus spin fluctuation rate $\nu$ given by Eq. (18) are shown for $LiV_2O_4$ (with $T \sim 10^1$ K). Note that the peak of $1/T^a_1T$ is observed at $\nu = \omega_a \equiv \gamma_a B$ ($\gamma_I = 1.0396 \times 10^8$ s$^{-1}$T$^{-1}$, $\gamma_\mu = 8.5156 \times 10^8$ s$^{-1}$T$^{-1}$), where the curves correspond to $B \simeq 0.1$ T. Solid curves represent the regions where $1/T^a_1$ is within the sensitive range of the respective probes, while those corresponding to dashed curves are virtually out of range.

| | $\mu$SR | NMR |
|---|---|---|
| Time window ($T_\mathrm{W}$) | $10^{-9} \le T_\mathrm{W} \le 10^{-5}$ [s] | $10^{-2} \le T_\mathrm{W}$ [s] |
| Fluctuation rate ($\nu$) | $10^4 \le \nu \le 10^{12}$ [s$^{-1}$] | $\nu \le 10^2, \nu \ge 10^{12}$ [s$^{-1}$] |

TABLE I. Sensitive ranges of spin fluctuation rate for $\mu$SR and $^7$Li-NMR predicted from Eq. (18). See Fig. S2 for more details.


[1] S. Das, X. Zong, A. Niazi, A. Ellern, J. Q. Yan, and D. C. Johnston, Crystallography, magnetic susceptibility, heat capacity, and electrical resistivity of heavy-fermion $LiV_2O_4$ single crystals grown using a self-flux technique, Phys. Rev. B **76**, 054418-1/6 (2007).

[2] Y. Matsushita, H. Ueda, and Y. Ueda, Flux Crystal Growth and Thermal Stabilities of $LiV_2O_4$, Nature Materials **4**, 845–850 (2005).

[3] Y. Matsushita, J. Yamaura, and Y. Ueda, Lithium divanadate spinel, $LiV_2O_4$, Acta Crystallogr. E **61**, 137–139 (2005).

[4] See, for example, A. Yaouanc, and P. Dalmas de Réotier, *Muon Spin Rotation, Relaxation and Resonance: Application to condensed Matter*, Oxford University Press, 2011.

[5] See, for example, C. P. Slichter, *Principles of Magnetic Resonance*, Springer, New York, 1990 3rd ed.
